# Supplementary material for: Investigating Vulnerabilities of GPS Trip Data to Trajectory-User Linking Attacks
Source: arXiv:2502.08217 source file (2025-02-12)
Supplement: Supplementary file 2 [file dataset.tex]

%TC:ignore
\begin{figure}[H]
    \centering
    \includegraphics[width=10cm]{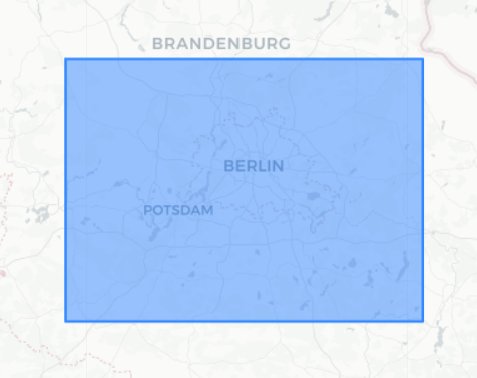}
    \caption{Bounding box of tesselation used for Berlin and the freemove dataset. Trajectories starting or ending outside of this box are discarded.}
    \label{Figure:boxberlin}
\end{figure}

\begin{figure}[H]
    \centering
    \includegraphics[width=10cm]{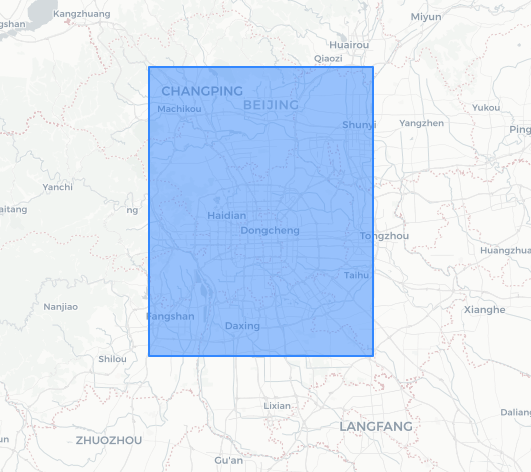}
    \caption{Bounding box of tesselation used for Beijing and the GeoLife dataset. Trajectories starting or ending outside of this box are discarded.}
    \label{Figure:boxpeking}
\end{figure}

%TC:endignore
