# Supplementary material for: Investigating Vulnerabilities of GPS Trip Data to Trajectory-User Linking Attacks
Source: arXiv:2502.08217 source file (2025-02-12)
Supplement: Supplementary file 4 [file methoddetails.tex]

%TC:ignore
\begin{figure}[H]
    \centering
    \includegraphics[width=\linewidth]{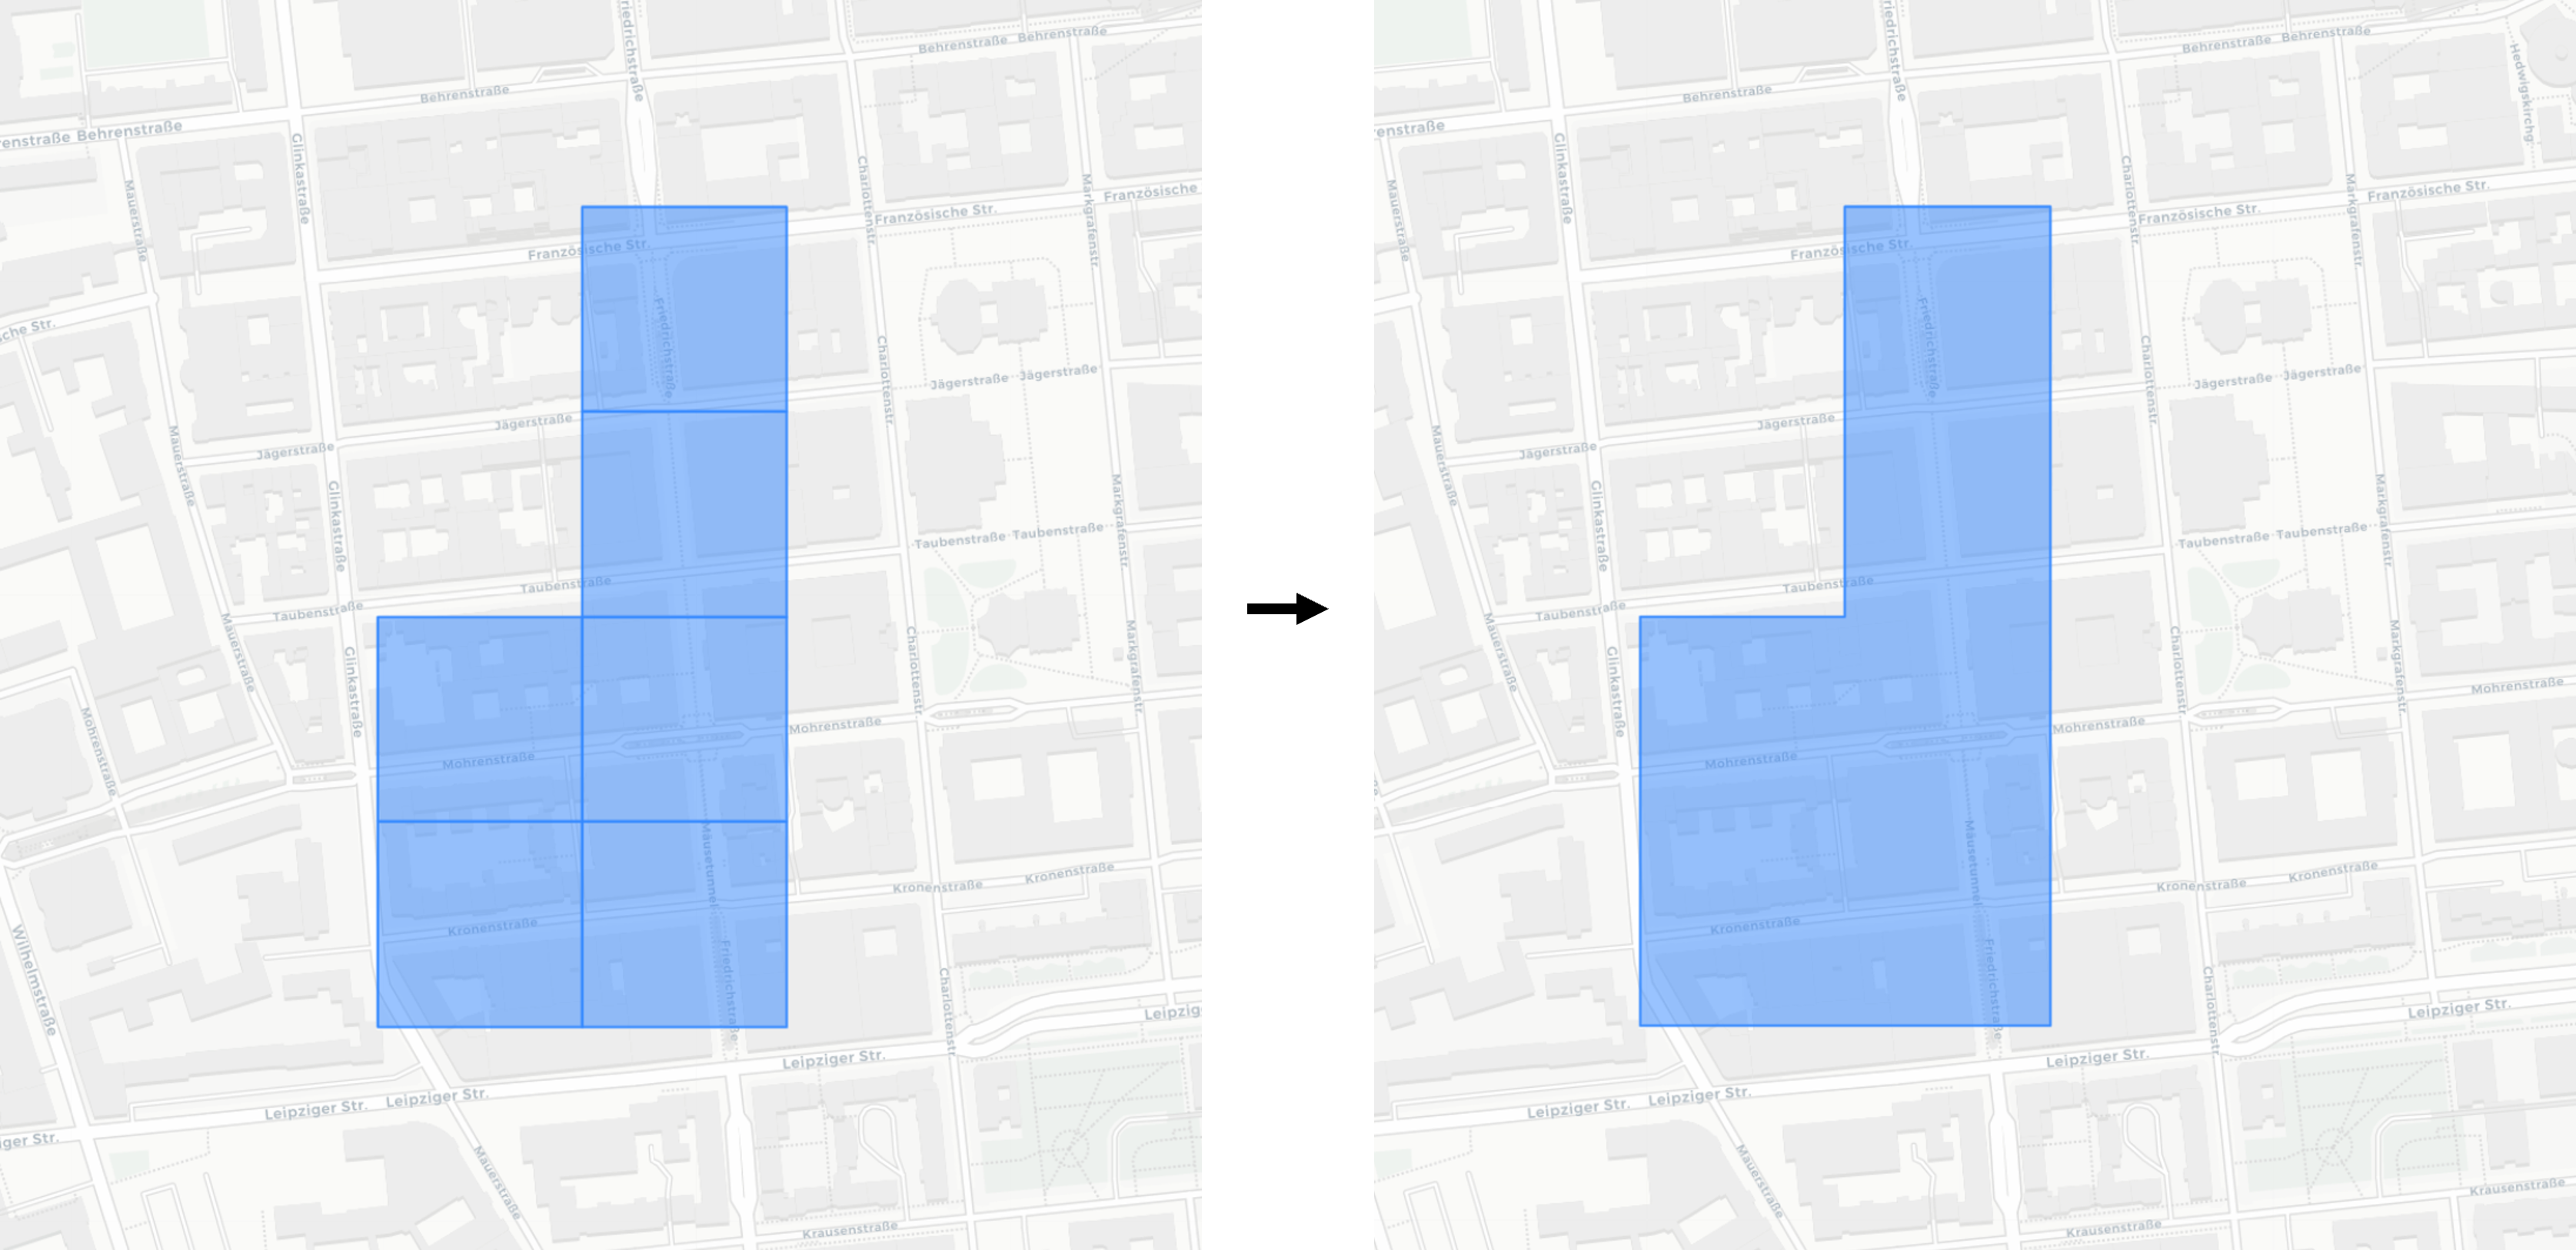}
    \caption{Example illustration of adjacent HL tiles that would be dissolved into one combined polygon during the HL assignment step.}
    \label{Figure:dissolvingexample}
\end{figure}

\begin{figure}[H]
    \centering
    \includegraphics[width=\linewidth]{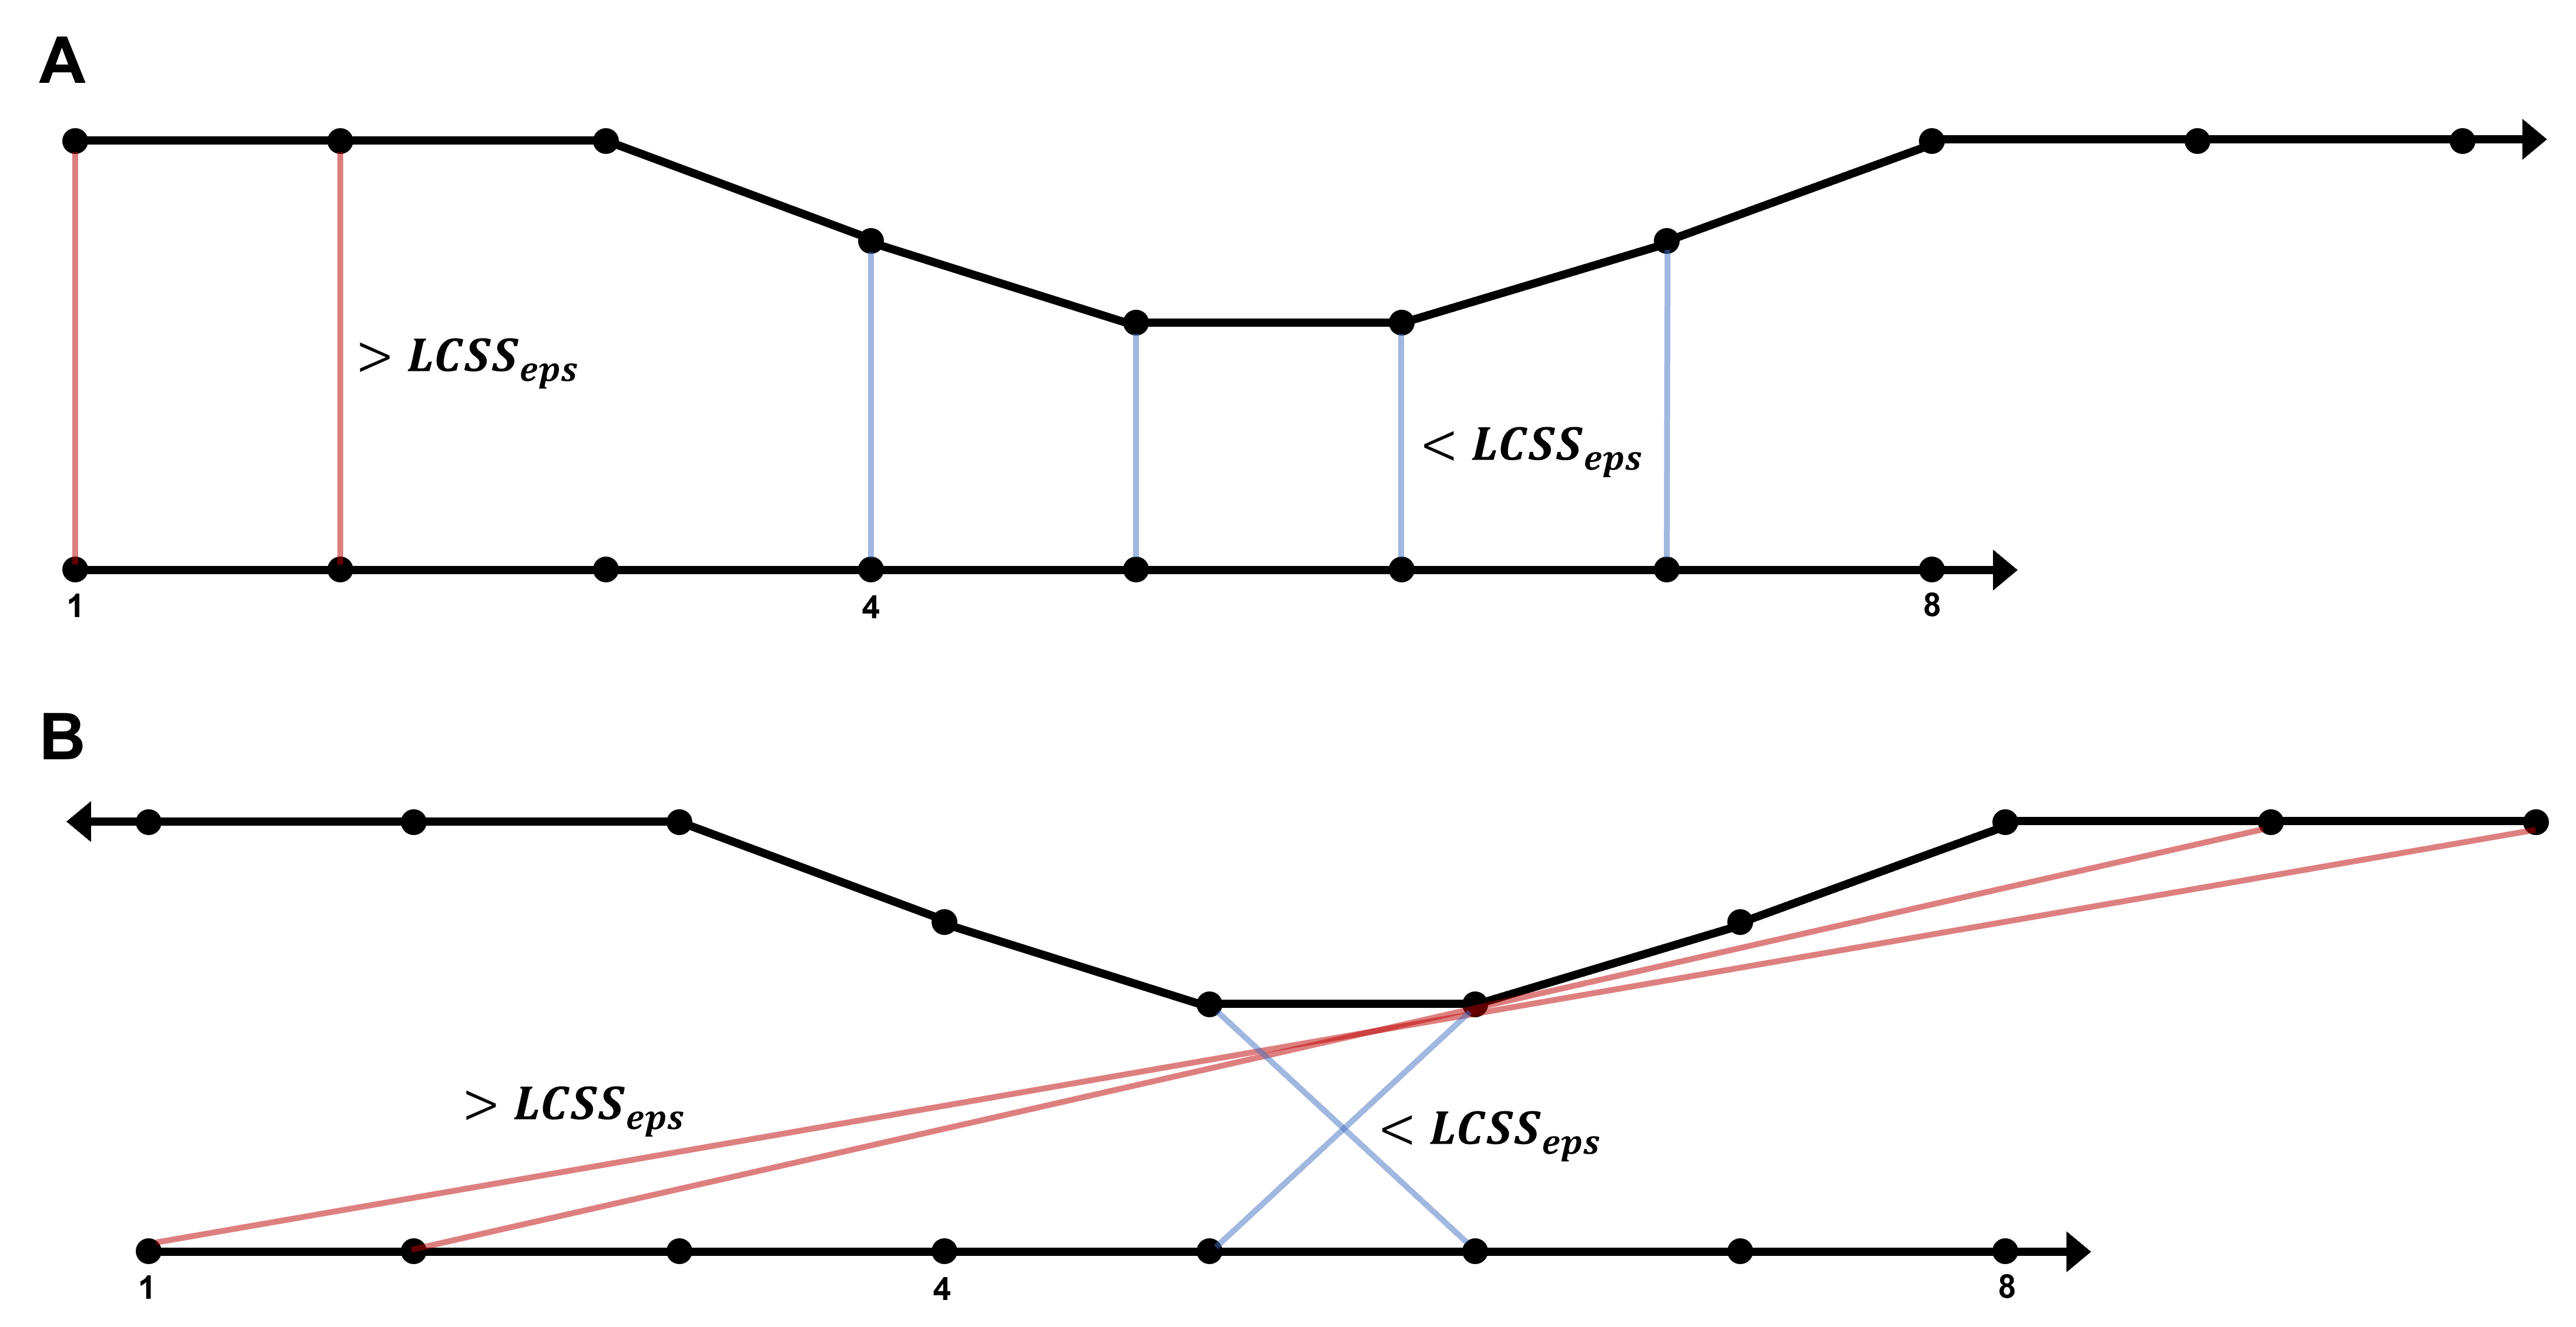}
    \caption{Example illustration of LCSS metric for a pair of trajectories. (A) being the original trips and (B) with the upper trajectory reverted. The LCSS value in (A) is 0.5 since 50\% of the points of the shorter trajectory are within a distance threshold $LCSS_{eps}$ from their counterpart in the longer trajectory. Analogously, in (B) the LCSS results in 0.25 because when comparing the points in reverted order -- the direction of travel for one of the trajectories goes in the opposite direction, only 25\% of the points are within $LCSS_{eps}$. Note here that for easier readability the red lines indicating points that are further apart than the specified threshold, are only plotted exemplary for two of the above point pairs.}
    \label{Figure:lcss}
\end{figure}

\subsubsection{Motivation for iterative TF-IDF refinement over standard clustering}\label{appendix:motivation_tfidf}

It is important to point out that I am not applying standard clustering techniques to the TF-IDF weighted location visit patterns to further refine our user ID mapping since the objective is not to find overall similar sets of trajectories but rather the highly relevant link that contains -- from an information-theoretic view -- high "amounts of information" \citep{aizawaInformationtheoreticPerspectiveTf2003}. In other words, this approach aims to link two otherwise disjoint sets of trajectories that reflect two behavior patterns of the same person. For example, instead of matching geospatially similar trips, such as all the commuters traveling to a business district starting in the same part of town, I identify if there is a trip connecting the HLs of an individual in our data and their hypothetical partner in case this person frequently stays over at their partner's apartment.

\begin{figure}[H]
    \centering
    \includegraphics[width=6cm]{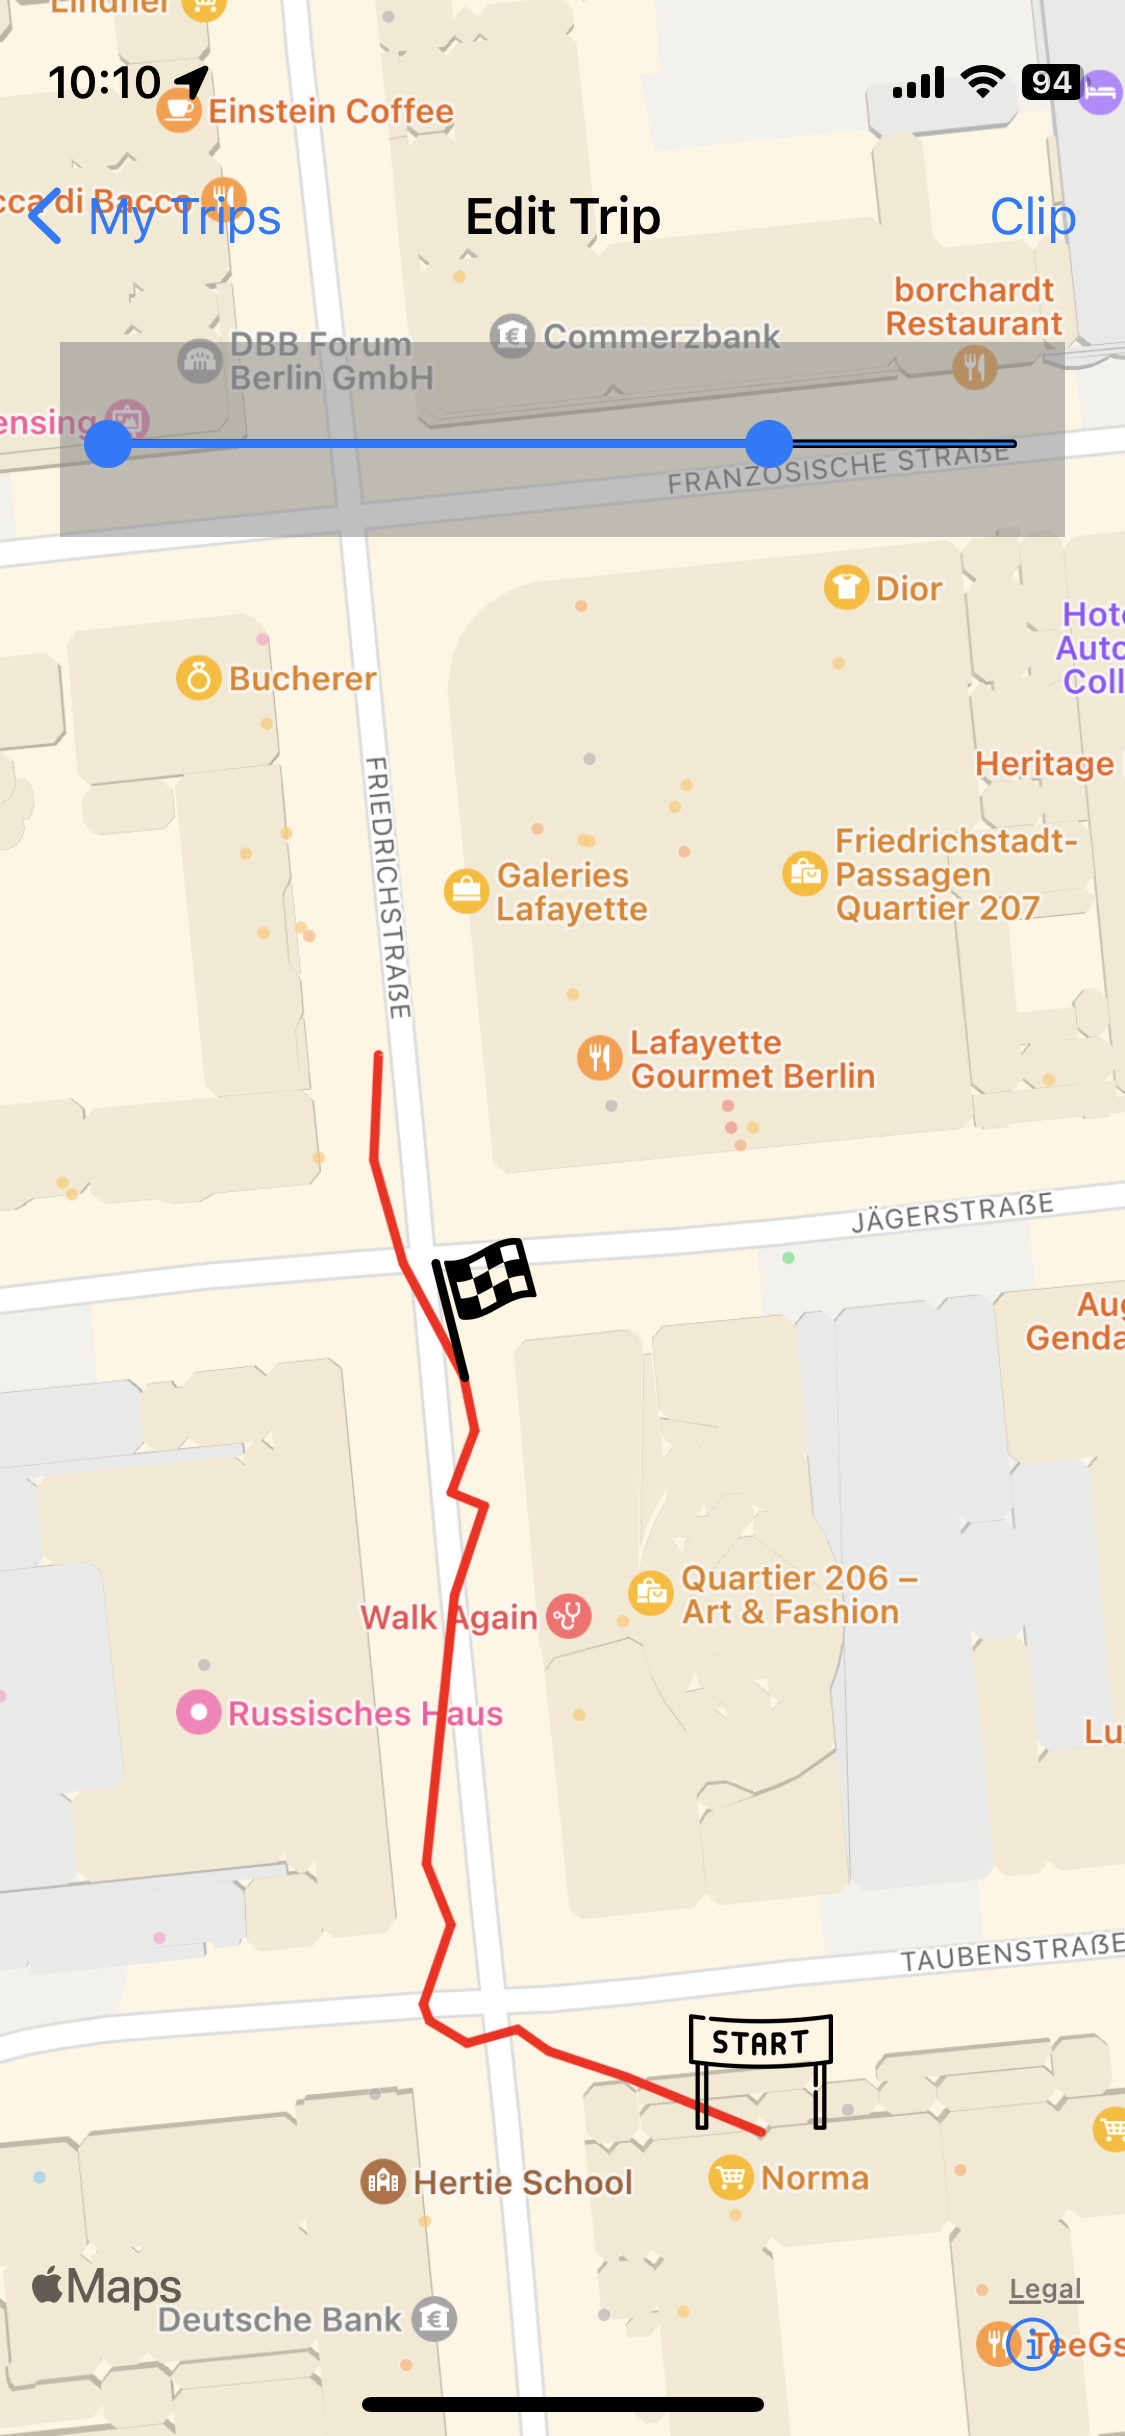}
    \caption{Screenshot of the SimRa app where users have the choice to truncate their trajectories by a variable margin set with a slider control around starting and end points.}
    \label{Figure:simratrip}
\end{figure}

\begin{figure}[H]
    \centering
    \includegraphics[width=6cm]{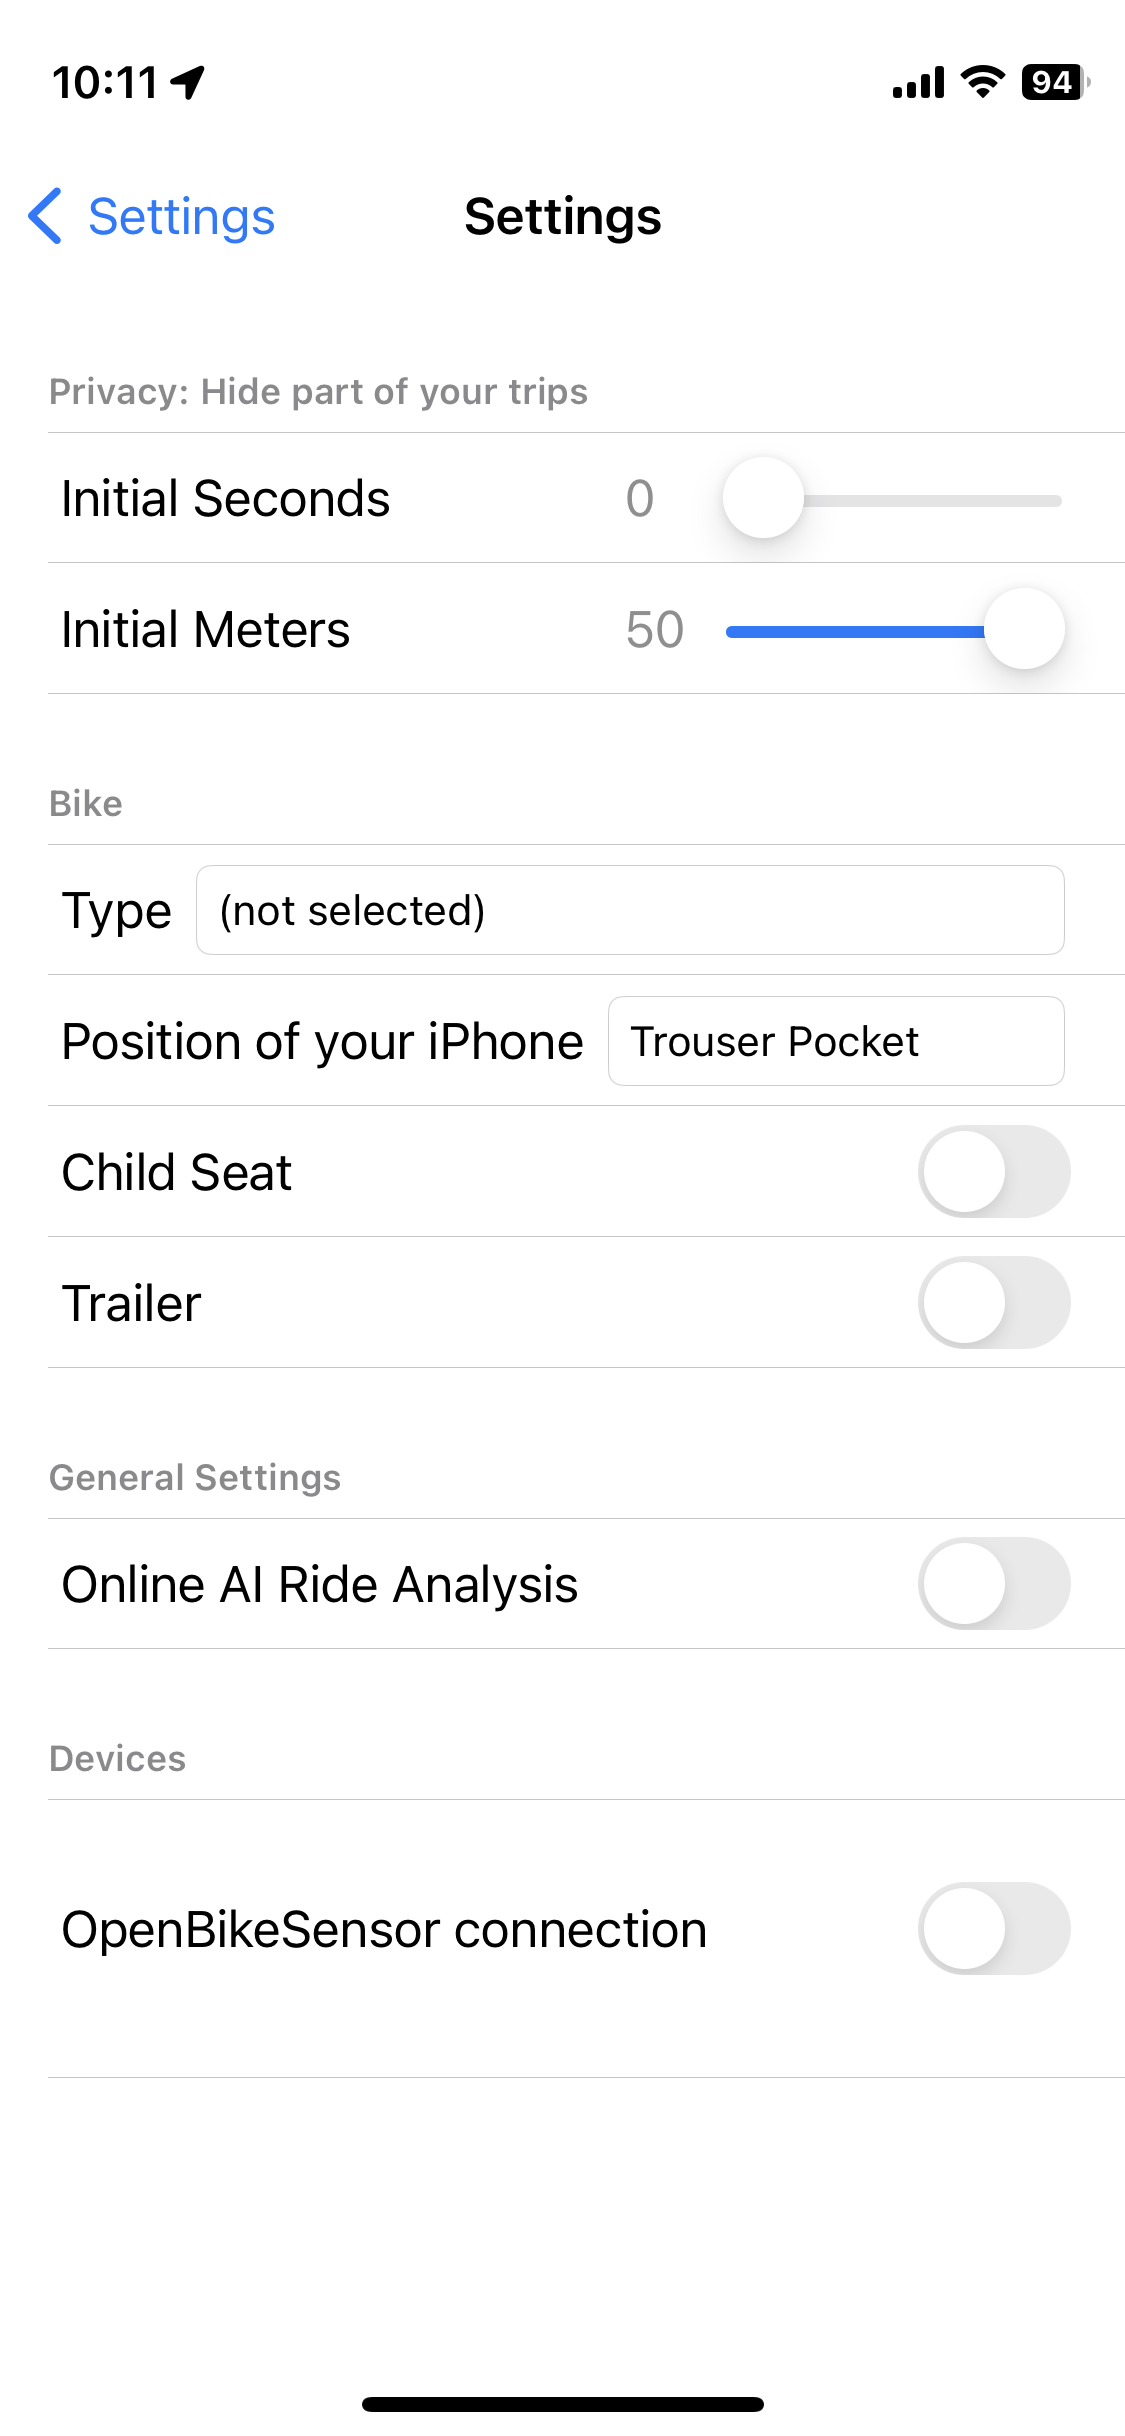}
    \caption{Screenshot of the SimRa app's preferences showing the setting for truncating an initial segment of flexible length up to 50m for every trajectory by default.}
    \label{Figure:simrasettings}
\end{figure}

%TC:endignore
